# Supplementary material for: Degree Centrality Algorithms For Homogeneous Multilayer Networks
Source: arXiv:2207.11661 source file (2022-07-24)
Supplement: Supplementary file 1 [file Appendices.tex]

\section{Appendix}
\label{sec:appendix}
\appendix

%%\textbf{Algorithm for Closeness Centrality Heuristic 1}

%%\textbf{Algorithm for Closeness Centrality Heuristic 2}
